# Supplementary material for: Calibration to American Options: Numerical Investigation of the de-Americanization
Source: arXiv:1611.06181 source file (2016-11-18)
Supplement: Supplementary file 1 [file appendix.tex]

\appendix
%\section{Scratch}
%\begin{itemize}
%\item 17.11 first version
%\item 08.12. second version
%\item 04.03 third version
%\begin{itemize}
% \item Section about Heston model updated
% \item Additonal references added
% \item Update regarding structure and results
%\end{itemize}
%
%\end{itemize}

\begin{table}[h]
\begin{center}
 \begin{tabular}{|c|c|c|c|c|c|}
 	\hline
Scenario&$\sigma$&$\rho$&r&maximum error&average error\\
\hline
1&0.3&0.8&0&	$1.8\cdot10^{-4}$	&	$3.6\cdot10^{-5}$\\
 	\hline
 	2&0.3&0.8&0.07&	1.1	&	$1.1\cdot10^{-1}$\\
 	\hline
 	3&0.5&0.8&0&	$1.6\cdot10^{-4}$	&	$4.3\cdot10^{-5}$\\
 	\hline
 	4&0.5&0.8&0.07&	$3.4\cdot10^{-1}$	&	$1.1\cdot10^{-1}$\\
 	\hline
 	5&	0.1&	0.8&	0&	$1.5\cdot10^{-4}$&	$1.7\cdot10^{-5}$\\
 	\hline
 	6	&0.1&	0.8	&0.07&	5.2	&	$4.3\cdot10^{-1}$\\
 	\hline
 	7&	0.3&	0.5&	0&	$1.3\cdot10^{-4}$	&	$2.3\cdot10^{-5}$\\
 	\hline
 	8&	0.3&	0.5&	0.07&	3.4	&	$3.0\cdot10^{-1}$\\
 	\hline
 	9&	0.5&	0.5&	0&	$2.0\cdot10^{-4}$	&	$3.9\cdot10^{-5}$\\
 	\hline
 	10&	0.5&	0.5&	0.07&	$5.8\cdot10^{-1}$	&	$5.1\cdot10^{-2}$\\
 	\hline
 	11&	0.1&	0.5&	0&	$3.6\cdot10^{-4}$	&	$1.5\cdot10^{-5}$\\
 	\hline
 	12&	0.1&	0.5&	0.07&	6.9	&	$6.1\cdot10^{-1}$\\
 	\hline
 	13&	0.3&	1&	0&	$1.9\cdot10^{-4}$	&	$4.7\cdot10^{-5}$\\
 	\hline
 	14&	0.3&	1&	0.07&	$3.5\cdot10^{-1}$	&	$9.8\cdot10^{-2}$\\
 	\hline
 	15&	0.5&	1&	0&	$2.2\cdot10^{-4}$	&	$6.1\cdot10^{-5}$\\
 	\hline
 	16&	0.5&	1&	0.07&	$5.9\cdot10^{-1}$	&	$1.6\cdot10^{-1}$\\
 	\hline
 	17&	0.1&	1&	0&	$1.2\cdot10^{-4}$	&	$2.1\cdot10^{-5}$\\
 	\hline
 	18&	0.1&	1&	0.07&	3.1	&	$2.9\cdot10^{-1}$\\
 	\hline
 \end{tabular}
 \caption{Processed Google option data for $t_0=\text{02.02.2015}$, $S_0=523.76$}
 \label{ScenCEV}
 \end{center}
\end{table}

\begin{table}[h]
\begin{center}
 \begin{tabular}{|c|c|c|c|c|c|c|c|c|}
 	\hline
 	Scenario&$\xi$&$\rho$&$\gamma$&$\kappa$&$v_0$&r&maximum error&average error\\
	\hline
	1	&	0.3	&	0	&	0.16	&	0.3	&	0.15	&	0.07&$1.6\cdot10^{-1}$	&	$2.7\cdot10^{-2}$	\\
	\hline
	2	&	0.3	&	0	&	0.16	&	0.3	&	0.15	&	0&	$3.0\cdot10^{-4}$	&	$4.5\cdot10^{-5}$	\\
	\hline
	3	&	0.3	&	0.9	&	0.16	&	0.3	&	0.15	&	0.07&	$3.9\cdot10^{-1}$	&	$7.9\cdot10^{-2}$	\\
	\hline
	4	&	0.3	&	0.9	&	0.16	&	0.3	&	0.15	&	0&	$2.8\cdot10^{-4}$	&	$5.3\cdot10^{-5}$	\\
	\hline
	5	&	0.3	&	0.5	&	0.16	&	0.3	&	0.15	&	0.07&	$3.1\cdot10^{-1}$	&	$5.7\cdot10^{-2}$	\\
	\hline
	6	&	0.3	&	0.5	&	0.16	&	0.3	&	0.15	&	0	&	$2.1\cdot10^{-4}$	&	$5.5\cdot10^{-5}$\\
	\hline
	7	&	0.3	&	-0.5	&	0.16	&	0.3	&	0.15	&	0.07&	$1.1\cdot10^{-1}$	&	$3.4\cdot10^{-2}$	\\
	\hline
	8	&	0.3	&	-0.5	&	0.16	&	0.3	&	0.15	&	0&	$2.1\cdot10^{-3}$	&	$2.0\cdot10^{-4}$	\\
	\hline
	9	&	0.3	&	-0.9	&	0.16	&	0.3	&	0.15	&	0.07&	$2.7\cdot10^{-1}$	&	$7.1\cdot10^{-2}$	\\
	\hline
	10	&	0.3	&	-0.9	&	0.16	&	0.3	&	0.15	&	0&	$1.2\cdot10^{-2}$	&	$1.1\cdot10^{-3}$	\\
	\hline
	11	&	0.6	&	-0.5	&	0.16	&	0.3	&	0.15	&	0.07&	$4.1\cdot10^{-1}$	&	$5.0\cdot10^{-2}$	\\
	\hline
	12	&	0.6	&	-0.5	&	0.16	&	0.3	&	0.15	&	0&	$1.1\cdot10^{-1}$	&	$1.3\cdot10^{-2}$	\\
	\hline
	13	&	0.1	&	-0.5	&	0.16	&	0.3	&	0.15	&	0.07&	$1.6\cdot10^{-1}$	&	$4.6\cdot10^{-2}$	\\
	\hline
	14	&	0.1	&	-0.5	&	0.16	&	0.3	&	0.15	&	0&	$2.3\cdot10^{-4}$	&	$5.3\cdot10^{-5}$	\\
	\hline
	15	&	0.3	&	0.5	&	0.1	&	0.3	&	0.15	&	0.07&	$6.0\cdot10^{-1}$	&	$9.4\cdot10^{-2}$	\\
	\hline
	16	&	0.3	&	-0.5	&	0.1	&	0.3	&	0.15	&	0&	$8.0\cdot10^{-3}$	&	$6.5\cdot10^{-4}$	\\
	\hline
	17	&	0.3	&	0.5	&	0.2	&	0.3	&	0.15	&	0.07&	$1.5\cdot10^{-1}$	&	$3.6\cdot10^{-2}$	\\
	\hline
	18	&	0.3	&	-0.5	&	0.2	&	0.3	&	0.15	&	0&	$6.2\cdot10^{-4}$	&	$8.4\cdot10^{-5}$	\\
	\hline
	19	&	0.3	&	-0.5	&	0.16	&	0.5	&	0.15	&	0.07&	$1.2\cdot10^{-1}$	&	$3.4\cdot10^{-2}$	\\
	\hline
	20	&	0.3	&	-0.5	&	0.16	&	0.5	&	0.15	&	0	&	$4.9\cdot10^{-4}$	&	$9.5\cdot10^{-5}$\\
	\hline
	21	&	0.3	&	-0.5	&	0.16	&	0.1	&	0.15	&	0.07&	$1.1\cdot10^{-1}$	&	$3.2\cdot10^{-2}$	\\
	\hline
	22	&	0.3	&	-0.5	&	0.16	&	0.1	&	0.15	&	0&	$1.1\cdot10^{-2}$	&	$8.2\cdot10^{-4}$	\\
	\hline
	23	&	0.3	&	-0.5	&	0.16	&	0.3	&	0.05	&	0.07&	$7.2\cdot10^{-1}$	&	$1.3\cdot10^{-1}$	\\
	\hline
	24	&	0.3	&	-0.5	&	0.16	&	0.3	&	0.05	&	0&	$4.1\cdot10^{-2}$	&	$1.9\cdot10^{-3}$	\\
	\hline
	25	&	0.3	&	-0.5	&	0.16	&	0.3	&	0.25	&	0.07&	$2.3\cdot10^{-1}$	&	$3.2\cdot10^{-2}$	\\
	\hline
	26	&	0.3	&	-0.5	&	0.16	&	0.3	&	0.25	&	0	&	$7.7\cdot10^{-4}$	&	$1.0\cdot10^{-4}$\\
	\hline
 	 \end{tabular}
 \caption{Processed Google option data for $t_0=\text{02.02.2015}$, $S_0=523.76$}
 \label{ScenHeston}
 \end{center}
\end{table}

\begin{figure}[h!]
\begin{center}
\includegraphics[width=0.9\textwidth]{fig/CEV_All_Mats.jpg}
\caption{Calibration results for the Google market data in the CEV model}
\label{CEV_Google_cali}
\end{center}
\end{figure}

\begin{figure}[h!]
\begin{center}
\includegraphics[width=0.9\textwidth]{fig/16Feb15_GoogleData_2015_processed_all_maturities_callput_RBM0_lsq.png}
\caption{Calibration results for the Google market data in the Heston model}
\label{Heston_Google_cali}
\end{center}
\end{figure}

\begin{figure}[H]
\centering
    \subfigure[\subcapsize Prices for Scenario 1]{
        %\label{error_cev_1} 
        \includegraphics[width=3cm]{./fig/Bilder_Pricing/CEV_Prices_1.png}}
            \hspace{0.1in}              
    \subfigure[Pricing differences - Scenario 1]{
        %\label{error_cev_2} 
        \includegraphics[width=3cm]{./fig/Bilder_Pricing/CEV_Differences_1.png}}         
        \hspace{0.1in}           
    \subfigure[Prices for Scenario 2]{
        %\label{error_cev_1} 
        \includegraphics[width=3cm]{./fig/Bilder_Pricing/CEV_Prices_2.png}}
       \hspace{0.1in}                
    \subfigure[Pricing differences - Scenario 2]{
        %\label{error_cev_2} 
        \includegraphics[width=3cm]{./fig/Bilder_Pricing/CEV_Differences_2.png}}         
                   \hspace{0.1in}               
    \subfigure[Prices for Scenario 3]{
        %\label{error_cev_1} 
        \includegraphics[width=3cm]{./fig/Bilder_Pricing/CEV_Prices_3.png}}
            \hspace{0.1in}
    \subfigure[Pricing differences - Scenario 3]{
        %\label{error_cev_2} 
        \includegraphics[width=3cm]{./fig/Bilder_Pricing/CEV_Differences_3.png}}         
        \hspace{0.1in}
    \subfigure[Prices for Scenario 4]{
        %\label{error_cev_1} 
        \includegraphics[width=3cm]{./fig/Bilder_Pricing/CEV_Prices_4.png}}
            \hspace{0.1in}
    \subfigure[Pricing differences - Scenario 4]{
        %\label{error_cev_2} 
        \includegraphics[width=3cm]{./fig/Bilder_Pricing/CEV_Differences_4.png}}         
               \hspace{0.1in}            
    \subfigure[Prices for Scenario 5]{
        %\label{error_cev_1} 
        \includegraphics[width=3cm]{./fig/Bilder_Pricing/CEV_Prices_5.png}}
            \hspace{0.1in}
    \subfigure[Pricing differences - Scenario 5]{
        %\label{error_cev_2} 
        \includegraphics[width=3cm]{./fig/Bilder_Pricing/CEV_Differences_5.png}}         
        \hspace{0.1in}                
    \subfigure[Prices for Scenario 6]{
        %\label{error_cev_1} 
        \includegraphics[width=3cm]{./fig/Bilder_Pricing/CEV_Prices_6.png}}
            \hspace{0.1in}
    \subfigure[Pricing differences - Scenario 6]{
        %\label{error_cev_2} 
        \includegraphics[width=3cm]{./fig/Bilder_Pricing/CEV_Differences_6.png}}         
               \hspace{0.1in}
    \subfigure[Prices for Scenario 7]{
        %\label{error_cev_1} 
        \includegraphics[width=3cm]{./fig/Bilder_Pricing/CEV_Prices_7.png}}
            \hspace{0.1in}
    \subfigure[Pricing differences - Scenario 7]{
        %\label{error_cev_2} 
        \includegraphics[width=3cm]{./fig/Bilder_Pricing/CEV_Differences_7.png}}         
        \hspace{0.1in}        
    \subfigure[Prices for Scenario 8]{
        %\label{error_cev_1} 
        \includegraphics[width=3cm]{./fig/Bilder_Pricing/CEV_Prices_8.png}}
            \hspace{0.1in}
    \subfigure[Pricing differences - Scenario 8]{
        %\label{error_cev_2} 
        \includegraphics[width=3cm]{./fig/Bilder_Pricing/CEV_Differences_8.png}}         
       \hspace{0.1in}      
    \subfigure[Prices for Scenario 9]{
        %\label{error_cev_1} 
        \includegraphics[width=3cm]{./fig/Bilder_Pricing/CEV_Prices_9.png}}
            \hspace{0.1in}
    \subfigure[Pricing differences - Scenario 9]{
        %\label{error_cev_2} 
        \includegraphics[width=3cm]{./fig/Bilder_Pricing/CEV_Differences_9.png}}         
        \hspace{0.1in}        
    \subfigure[Prices for Scenario 10]{
        %\label{error_cev_1} 
        \includegraphics[width=3cm]{./fig/Bilder_Pricing/CEV_Prices_10.png}}
            \hspace{0.1in}
    \subfigure[Pricing differences - Scenario 10]{
        %\label{error_cev_2} 
        \includegraphics[width=3cm]{./fig/Bilder_Pricing/CEV_Differences_10.png}}         
       \hspace{0.1in}
 \subfigure[Prices for Scenario 11]{
        %\label{error_cev_1} 
        \includegraphics[width=3cm]{./fig/Bilder_Pricing/CEV_Prices_11.png}}
            \hspace{0.1in}
    \subfigure[Pricing differences - Scenario 11]{
        %\label{error_cev_2} 
        \includegraphics[width=3cm]{./fig/Bilder_Pricing/CEV_Differences_11.png}}         
        \hspace{0.1in}
    \subfigure[Prices for Scenario 12]{
        %\label{error_cev_1} 
        \includegraphics[width=3cm]{./fig/Bilder_Pricing/CEV_Prices_12.png}}
            \hspace{0.1in}
    \subfigure[Pricing differences - Scenario 12]{
        %\label{error_cev_2} 
        \includegraphics[width=3cm]{./fig/Bilder_Pricing/CEV_Differences_12.png}}         
        \hspace{0.1in}

\caption{CEV 1-10} 
\label{Results_CEV_1}
\end{figure}

\begin{figure}[H]
\centering     
        \subfigure[Prices for Scenario 13]{
        %\label{error_cev_1} 
        \includegraphics[width=3cm]{./fig/Bilder_Pricing/CEV_Prices_13.png}}
            \hspace{0.1in}
    \subfigure[Pricing differences - Scenario 13]{
        %\label{error_cev_2} 
        \includegraphics[width=3cm]{./fig/Bilder_Pricing/CEV_Differences_13.png}}         
        \hspace{0.1in}    
    \subfigure[Prices for Scenario 14]{
        %\label{error_cev_1} 
        \includegraphics[width=3cm]{./fig/Bilder_Pricing/CEV_Prices_14.png}}
            \hspace{0.1in}
    \subfigure[Pricing differences - Scenario 14]{
        %\label{error_cev_2} 
        \includegraphics[width=3cm]{./fig/Bilder_Pricing/CEV_Differences_14.png}}  
           \hspace{0.1in}                  
    \subfigure[Prices for Scenario 15]{
        %\label{error_cev_1} 
        \includegraphics[width=3cm]{./fig/Bilder_Pricing/CEV_Prices_15.png}}
            \hspace{0.1in}
    \subfigure[Pricing differences - Scenario 15]{
        %\label{error_cev_2} 
        \includegraphics[width=3cm]{./fig/Bilder_Pricing/CEV_Differences_15.png}}         
        \hspace{0.1in}                
    \subfigure[Prices for Scenario 16]{
        %\label{error_cev_1} 
        \includegraphics[width=3cm]{./fig/Bilder_Pricing/CEV_Prices_16.png}}
            \hspace{0.1in}
    \subfigure[Pricing differences - Scenario 16]{
        %\label{error_cev_2} 
        \includegraphics[width=3cm]{./fig/Bilder_Pricing/CEV_Differences_16.png}}         
        \hspace{0.1in}
    \subfigure[Prices for Scenario 17]{
        %\label{error_cev_1} 
        \includegraphics[width=3cm]{./fig/Bilder_Pricing/CEV_Prices_17.png}}
            \hspace{0.1in}
    \subfigure[Pricing differences - Scenario 17]{
        %\label{error_cev_2} 
        \includegraphics[width=3cm]{./fig/Bilder_Pricing/CEV_Differences_17.png}}         
        \hspace{0.1in}        
    \subfigure[Prices for Scenario 18]{
        %\label{error_cev_1} 
        \includegraphics[width=3cm]{./fig/Bilder_Pricing/CEV_Prices_18.png}}
            \hspace{0.1in}
    \subfigure[Pricing differences - Scenario 18]{
        %\label{error_cev_2} 
        \includegraphics[width=3cm]{./fig/Bilder_Pricing/CEV_Differences_18.png}}         
        \hspace{0.1in}      
       
\caption{CEV 11-18} 
\label{Results_CEV_2}
\end{figure}
\begin{figure}[H]
\centering
    \subfigure[Prices for Scenario 1]{
        %\label{error_cev_1} 
        \includegraphics[width=3cm]{./fig/Bilder_Pricing/Heston_Prices_1.png}}
            \hspace{0.1in}
    \subfigure[Pricing differences - Scenario 1]{
        %\label{error_cev_2} 
        \includegraphics[width=3cm]{./fig/Bilder_Pricing/Heston_Differences_1.png}}         
        \hspace{0.1in}
    \subfigure[Prices for Scenario 2]{
        %\label{error_cev_1} 
        \includegraphics[width=3cm]{./fig/Bilder_Pricing/Heston_Prices_2.png}}
            \hspace{0.1in}
    \subfigure[Pricing differences - Scenario 2]{
        %\label{error_cev_2} 
        \includegraphics[width=3cm]{./fig/Bilder_Pricing/Heston_Differences_2.png}}         
        \hspace{0.1in}
    \subfigure[Prices for Scenario 3]{
        %\label{error_cev_1} 
        \includegraphics[width=3cm]{./fig/Bilder_Pricing/Heston_Prices_3.png}}
            \hspace{0.1in}
    \subfigure[Pricing differences - Scenario 3]{
        %\label{error_cev_2} 
        \includegraphics[width=3cm]{./fig/Bilder_Pricing/Heston_Differences_3.png}}         
        \hspace{0.1in}
    \subfigure[Prices for Scenario 4]{
        %\label{error_cev_1} 
        \includegraphics[width=3cm]{./fig/Bilder_Pricing/Heston_Prices_4.png}}
            \hspace{0.1in}
    \subfigure[Pricing differences - Scenario 4]{
        %\label{error_cev_2} 
        \includegraphics[width=3cm]{./fig/Bilder_Pricing/Heston_Differences_4.png}}         
        \hspace{0.1in}                
    \subfigure[Prices for Scenario 5]{
        %\label{error_cev_1} 
        \includegraphics[width=3cm]{./fig/Bilder_Pricing/Heston_Prices_5.png}}
            \hspace{0.1in}
    \subfigure[Pricing differences - Scenario 5]{
        %\label{error_cev_2} 
        \includegraphics[width=3cm]{./fig/Bilder_Pricing/Heston_Differences_5.png}}         
        \hspace{0.1in}                
    \subfigure[Prices for Scenario 6]{
        %\label{error_cev_1} 
        \includegraphics[width=3cm]{./fig/Bilder_Pricing/Heston_Prices_6.png}}
            \hspace{0.1in}
    \subfigure[Pricing differences - Scenario 6]{
        %\label{error_cev_2} 
        \includegraphics[width=3cm]{./fig/Bilder_Pricing/Heston_Differences_6.png}}         
        \hspace{0.1in}
    \subfigure[Prices for Scenario 7]{
        %\label{error_cev_1} 
        \includegraphics[width=3cm]{./fig/Bilder_Pricing/Heston_Prices_7.png}}
            \hspace{0.1in}
    \subfigure[Pricing differences - Scenario 7]{
        %\label{error_cev_2} 
        \includegraphics[width=3cm]{./fig/Bilder_Pricing/Heston_Differences_7.png}}         
        \hspace{0.1in}        
    \subfigure[Prices for Scenario 8]{
        %\label{error_cev_1} 
        \includegraphics[width=3cm]{./fig/Bilder_Pricing/Heston_Prices_8.png}}
            \hspace{0.1in}
    \subfigure[Pricing differences - Scenario 8]{
        %\label{error_cev_2} 
        \includegraphics[width=3cm]{./fig/Bilder_Pricing/Heston_Differences_8.png}}         
        \hspace{0.1in}        
    \subfigure[Prices for Scenario 9]{
        %\label{error_cev_1} 
        \includegraphics[width=3cm]{./fig/Bilder_Pricing/Heston_Prices_9.png}}
            \hspace{0.1in}
    \subfigure[Pricing differences - Scenario 9]{
        %\label{error_cev_2} 
        \includegraphics[width=3cm]{./fig/Bilder_Pricing/Heston_Differences_9.png}}         
        \hspace{0.1in}        
    \subfigure[Prices for Scenario 10]{
        %\label{error_cev_1} 
        \includegraphics[width=3cm]{./fig/Bilder_Pricing/Heston_Prices_10.png}}
            \hspace{0.1in}
    \subfigure[Pricing differences - Scenario 10]{
        %\label{error_cev_2} 
        \includegraphics[width=3cm]{./fig/Bilder_Pricing/Heston_Differences_10.png}}         
        \hspace{0.1in}              
\caption{Heston 1-10} 
\label{Results_Heston_1}
\end{figure}

\begin{figure}[H]
\centering
    \subfigure[Prices for Scenario 11]{
        %\label{error_cev_1} 
        \includegraphics[width=3cm]{./fig/Bilder_Pricing/Heston_Prices_11.png}}
            \hspace{0.1in}
    \subfigure[Pricing differences - Scenario 11]{
        %\label{error_cev_2} 
        \includegraphics[width=3cm]{./fig/Bilder_Pricing/Heston_Differences_11.png}}         
        \hspace{0.1in}
    \subfigure[Prices for Scenario 12]{
        %\label{error_cev_1} 
        \includegraphics[width=3cm]{./fig/Bilder_Pricing/Heston_Prices_12.png}}
            \hspace{0.1in}
    \subfigure[Pricing differences - Scenario 12]{
        %\label{error_cev_2} 
        \includegraphics[width=3cm]{./fig/Bilder_Pricing/Heston_Differences_12.png}}         
        \hspace{0.1in}
    \subfigure[Prices for Scenario 13]{
        %\label{error_cev_1} 
        \includegraphics[width=3cm]{./fig/Bilder_Pricing/Heston_Prices_13.png}}
            \hspace{0.1in}
    \subfigure[Pricing differences - Scenario 13]{
        %\label{error_cev_2} 
        \includegraphics[width=3cm]{./fig/Bilder_Pricing/Heston_Differences_13.png}}         
        \hspace{0.1in}
    \subfigure[Prices for Scenario 14]{
        %\label{error_cev_1} 
        \includegraphics[width=3cm]{./fig/Bilder_Pricing/Heston_Prices_14.png}}
            \hspace{0.1in}
    \subfigure[Pricing differences - Scenario 14]{
        %\label{error_cev_2} 
        \includegraphics[width=3cm]{./fig/Bilder_Pricing/Heston_Differences_14.png}}         
        \hspace{0.1in}                
    \subfigure[Prices for Scenario 15]{
        %\label{error_cev_1} 
        \includegraphics[width=3cm]{./fig/Bilder_Pricing/Heston_Prices_15.png}}
            \hspace{0.1in}
    \subfigure[Pricing differences - Scenario 15]{
        %\label{error_cev_2} 
        \includegraphics[width=3cm]{./fig/Bilder_Pricing/Heston_Differences_15.png}}         
        \hspace{0.1in}                
    \subfigure[Prices for Scenario 16]{
        %\label{error_cev_1} 
        \includegraphics[width=3cm]{./fig/Bilder_Pricing/Heston_Prices_16.png}}
            \hspace{0.1in}
    \subfigure[Pricing differences - Scenario 16]{
        %\label{error_cev_2} 
        \includegraphics[width=3cm]{./fig/Bilder_Pricing/Heston_Differences_16.png}}         
        \hspace{0.1in}
    \subfigure[Prices for Scenario 17]{
        %\label{error_cev_1} 
        \includegraphics[width=3cm]{./fig/Bilder_Pricing/Heston_Prices_17.png}}
            \hspace{0.1in}
    \subfigure[Pricing differences - Scenario 17]{
        %\label{error_cev_2} 
        \includegraphics[width=3cm]{./fig/Bilder_Pricing/Heston_Differences_17.png}}         
        \hspace{0.1in}        
    \subfigure[Prices for Scenario 18]{
        %\label{error_cev_1} 
        \includegraphics[width=3cm]{./fig/Bilder_Pricing/Heston_Prices_18.png}}
            \hspace{0.1in}
    \subfigure[Pricing differences - Scenario 18]{
        %\label{error_cev_2} 
        \includegraphics[width=3cm]{./fig/Bilder_Pricing/Heston_Differences_18.png}}         
        \hspace{0.1in}        
    \subfigure[Prices for Scenario 19]{
        %\label{error_cev_1} 
        \includegraphics[width=3cm]{./fig/Bilder_Pricing/Heston_Prices_19.png}}
            \hspace{0.1in}
    \subfigure[Pricing differences - Scenario 19]{
        %\label{error_cev_2} 
        \includegraphics[width=3cm]{./fig/Bilder_Pricing/Heston_Differences_19.png}}         
        \hspace{0.1in}        
    \subfigure[Prices for Scenario 20]{
        %\label{error_cev_1} 
        \includegraphics[width=3cm]{./fig/Bilder_Pricing/Heston_Prices_20.png}}
            \hspace{0.1in}
    \subfigure[Pricing differences - Scenario 20]{
        %\label{error_cev_2} 
        \includegraphics[width=3cm]{./fig/Bilder_Pricing/Heston_Differences_20.png}}         
        \hspace{0.1in}              
\caption{Heston 11-20} 
\label{Results_Heston_2}
\end{figure}

\begin{figure}[H]
\centering
    \subfigure[Prices for Scenario 21]{
        %\label{error_cev_1} 
        \includegraphics[width=3cm]{./fig/Bilder_Pricing/Heston_Prices_21.png}}
            \hspace{0.1in}
    \subfigure[Pricing differences - Scenario 21]{
        %\label{error_cev_2} 
        \includegraphics[width=3cm]{./fig/Bilder_Pricing/Heston_Differences_21.png}}         
        \hspace{0.1in}
    \subfigure[Prices for Scenario 22]{
        %\label{error_cev_1} 
        \includegraphics[width=3cm]{./fig/Bilder_Pricing/Heston_Prices_22.png}}
            \hspace{0.1in}
    \subfigure[Pricing differences - Scenario 22]{
        %\label{error_cev_2} 
        \includegraphics[width=3cm]{./fig/Bilder_Pricing/Heston_Differences_22.png}}         
        \hspace{0.1in}
    \subfigure[Prices for Scenario 23]{
        %\label{error_cev_1} 
        \includegraphics[width=3cm]{./fig/Bilder_Pricing/Heston_Prices_23.png}}
            \hspace{0.1in}
    \subfigure[Pricing differences - Scenario 23]{
        %\label{error_cev_2} 
        \includegraphics[width=3cm]{./fig/Bilder_Pricing/Heston_Differences_23.png}}         
        \hspace{0.1in}
    \subfigure[Prices for Scenario 24]{
        %\label{error_cev_1} 
        \includegraphics[width=3cm]{./fig/Bilder_Pricing/Heston_Prices_24.png}}
            \hspace{0.1in}
    \subfigure[Pricing differences - Scenario 24]{
        %\label{error_cev_2} 
        \includegraphics[width=3cm]{./fig/Bilder_Pricing/Heston_Differences_24.png}}         
        \hspace{0.1in}                
    \subfigure[Prices for Scenario 25]{
        %\label{error_cev_1} 
        \includegraphics[width=3cm]{./fig/Bilder_Pricing/Heston_Prices_25.png}}
            \hspace{0.1in}
    \subfigure[Pricing differences - Scenario 25]{
        %\label{error_cev_2} 
        \includegraphics[width=3cm]{./fig/Bilder_Pricing/Heston_Differences_25.png}}         
        \hspace{0.1in}                
    \subfigure[Prices for Scenario 26]{
        %\label{error_cev_1} 
        \includegraphics[width=3cm]{./fig/Bilder_Pricing/Heston_Prices_26.png}}
            \hspace{0.1in}
    \subfigure[Pricing differences - Scenario 26]{
        %\label{error_cev_2} 
        \includegraphics[width=3cm]{./fig/Bilder_Pricing/Heston_Differences_26.png}}         
        \hspace{0.1in}
           
\caption{Heston 21-26} 
\label{Results_Heston_3}
\end{figure}
